# Supplementary material for: The AI Economist: Optimal Economic Policy Design via Two-level Deep Reinforcement Learning
Source: arXiv:2108.02755 source file (2021-08-05)
Supplement: Supplementary file 1 [file supplementary.tex]

\hypertarget{supplementary-information}{
    \section{
    Supplementary Information
    }\label{supplementary-information}
}
